# Supplementary material for: Academic Performance and Behavioral Patterns
Source: arXiv:1706.09245 ancillary file (2018-04-09)
Supplement: Supplementary file 1 [file SI.pdf]

# Supporting Information

## A Student population

The investigated sample of students is part of a bigger population at the Technical University of Denmark (DTU). While there are about 11 000 enrolled students at DTU, we focused only on students of two cohort years, enrolled at the main campus (Lyngby campus). This leaves a student population of about 3 300 students. Out of these, about 1 000 students participated in the CNS and received a phone. For about half of it (538 students) we were able to collect complete data from all investigated channels enabling us to perform a thorough analysis. About 57% of them were in their first year and 35% in their second year at the beginning of the study, enrolled into 24 different majors (study-lines). Table 1 provides further information about the investigated sample as well as the considered student population. We see that the investigated sample has a slightly higher GPA as well as a lower proportion of women than the overall student population.

| | **Sample** | **Population** |
|---|---|---|
| *Size* | 538 | 3 339 |
| *Male/Female ratio* | 78% / 22% | 73% / 27% |
| *Mean GPA* | 2.5 | 2.15 |

**Table 1 Population overview** Sample vs. considered student population.

## B Interaction-based networks

Based on the the nature of the social interaction (proximity, Facebook, calls, and text messages) network ties were treated differently. Calls and text messages were reduced to unweighted relationships, as these interactions show insignificant variations over the pairs of students. On the contrary, network links based on physical proximity ("Face-to-face" meetings) and Facebook interactions were weighted by a non-linear scaling function to remove large deviations caused by the high usage frequency. The link weight $w'_{ij}$ is determined by

$$w'_{ij} = \lfloor \sqrt{w_{ij}} \rfloor, \tag{1}$$

where $w_{ij}$ denotes the original number of interactions between students $i$ and $j$. All interactions are considered as undirected, that is, social ties are symmetric.

## C Centrality measures

Centrality measures provide information about one's position in a network. For each network we evaluate the correlation of different centrality measures with the cumulative GPAs. Table 2 shows the resulting Spearman rank correlation coefficients. Overall, degree centrality displays the strongest correlation indicating that the number of social contacts plays an important role.

## D Permutation test

To test the significance of our observations regarding network ties, we have performed a permutation test. In this test we have randomly shuffled the node attributes (GPAs) in our network and see whether certain

| **Channel** | **Degree** | **Eigenvector** | **Closeness** | **Betweenness** | **Katz** | **Communicability** |
|---|---|---|---|---|---|---|
| *Calls* | 0.208 | 0.157 | 0.200 | 0.144 | 0.034 | 0.170 |
| *Texts* | 0.184 | 0.138 | 0.161 | 0.145 | 0.041 | 0.105 |
| *Proximity* | 0.255 | 0.246 | 0.248 | 0.241 | -0.042 | 0.246 |
| *FB Friends* | 0.143 | 0.143 | 0.146 | 0.068 | 0.011 | 0.142 |
| *FB interactions* | 0.143 | 0.127 | 0.137 | 0.071 | -0.008 | 0.127 |

**Table 2 Centrality measures** Correlations of different centrality measures and different channels with the cumulative GPAs.

effects disappear. In particular, we show that the magnitude of the correlation between the individual GPAs and the mean GPAs of the ego-network from text messages is significantly lower in the randomized networks than in the original one. The result after 1 000 runs is illustrated in Figure 1. There the true correlation coefficient $r_s$ exceeds the random observation by 5.42 standard deviations. This clearly indicates that the observed correlation between GPA and neighbors' GPA is not due to network structure.

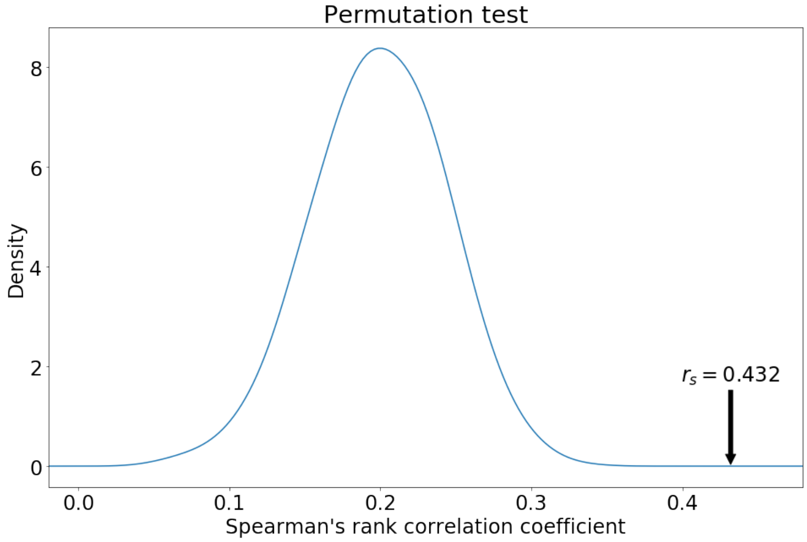


**Figure 1 Permutation test.** The blue curve shows the distribution of Spearman correlations between own performance and mean performance of the peer network with randomly shuffled GPAs. The observed correlation coefficients range between 0.063 and 0.331; significantly lower than 0.432 in the original network. The true value $r_s$ exceeds the random observation by 5.42 standard deviations.

The result of the permutation test is consistent with performing reshuffling of GPA with the entire student population, i.e. all using the GPA all those students who were eligible for enrolling in the study (irrespective of whether or not they participated in CNS).

# E Features

Table 3 gives an overview over all investigated features and provides some basics statistics describing the value distribution. It also contains the cumulative GPA which is the target in the supervised learning experiment. We can see here that the GPAs range from 0.38 to 3.96. That is, there are no students which have exclusively obtained 12s (best grade) or failing grades. On the contrary, for the class attendance feature we find students that did not show up to a single class as well as students that did not miss one.

| Feature set | | Feature | Mean | Median | Min | Max | Std |
|---|---|---|---|---|---|---|---|
| Target | | Cumulative GPA | 2.50 | 2.50 | 0.38 | 3.96 | 0.74 |
| Individual | Personality | PANAS (positive) | 14.95 | 15.00 | 9.00 | 20.00 | 2.10 |
| | | PANAS (negative) | 7.38 | 7.00 | 5.00 | 14.00 | 1.78 |
| | | Big Five: Openness | 3.53 | 3.60 | 2.20 | 4.80 | 0.50 |
| | | Big Five: Extraversion | 3.44 | 3.50 | 1.50 | 5.00 | 0.67 |
| | | Big Five: Neuroticism | 2.40 | 2.38 | 1.00 | 4.25 | 0.63 |
| | | Big Five: Agreeableness | 3.79 | 3.78 | 2.22 | 5.00 | 0.45 |
| | | Big Five: Conscientiousness | 3.44 | 3.44 | 1.89 | 4.89 | 0.56 |
| | | Satisfaction with Life | 27.60 | 28.00 | 5.00 | 35.00 | 5.34 |
| | | Self Esteem | 22.30 | 22.00 | 1.00 | 30.00 | 4.80 |
| | | Locus of Control | 5.11 | 5.00 | 0.00 | 12.00 | 2.27 |
| | | Narcissism: Admiration | 10.12 | 10.00 | 3.67 | 16.33 | 2.19 |
| | | Narcissism: Rivalry | 6.46 | 6.33 | 3.00 | 13.00 | 1.94 |
| | | Narcissism: Overall | 8.29 | 8.33 | 3.33 | 13.33 | 1.66 |
| | | Depression | 9.06 | 8.00 | 0.00 | 35.00 | 5.96 |
| | | Stress | 12.55 | 12.00 | 0.00 | 31.00 | 5.45 |
| | | Loneliness | 36.13 | 35.00 | 22.00 | 57.00 | 6.74 |
| | | Facebook Activity | -0.09 | -0.04 | -2.71 | 2.50 | 1.01 |
| | | Class Attendance | 0.71 | 0.76 | 0.00 | 1.00 | 0.20 |
| | | Gender | 0.78 | 1.00 | 0.00 | 1.00 | 0.42 |
| | | Study Year | 1.51 | 1.00 | 1.00 | 3.00 | 0.64 |
| Network | Calls | Mean GPA | 2.48 | 2.52 | 0.44 | 3.77 | 0.49 |
| | | Centrality | 0.01 | 0.01 | 0.00 | 0.07 | 0.01 |
| | | Low performing peers | 0.34 | 0.30 | 0.00 | 1.00 | 0.30 |
| | | High performing peers | 0.33 | 0.33 | 0.00 | 1.00 | 0.26 |
| | Texts | Mean GPA | 2.48 | 2.53 | 0.44 | 3.68 | 0.45 |
| | | Centrality | 0.01 | 0.01 | 0.00 | 0.06 | 0.01 |
| | | Low performing peers | 0.34 | 0.33 | 0.00 | 1.00 | 0.28 |
| | | High performing peers | 0.32 | 0.33 | 0.00 | 1.00 | 0.25 |
| | Proximity | Mean GPA | 2.52 | 2.53 | 2.25 | 2.76 | 0.07 |
| | | Centrality | 0.19 | 0.18 | 0.00 | 0.53 | 0.12 |
| | | Low performing peers | 0.35 | 0.36 | 0.27 | 0.39 | 0.01 |
| | | High performing peers | 0.33 | 0.33 | 0.30 | 0.41 | 0.01 |
| | Facebook interactions | Mean GPA | 2.50 | 2.51 | 0.99 | 3.26 | 0.31 |
| | | Centrality | 0.02 | 0.02 | 0.00 | 0.11 | 0.02 |
| | | Low performing peers | 0.33 | 0.33 | 0.00 | 1.00 | 0.19 |
| | | High performing peers | 0.33 | 0.33 | 0.00 | 1.00 | 0.17 |
| | Facebook friendships | Mean GPA | 2.47 | 2.48 | 0.93 | 3.31 | 0.26 |
| | | Centrality | 0.03 | 0.03 | 0.00 | 0.18 | 0.02 |
| | | Low performing peers | 0.34 | 0.33 | 0.00 | 1.00 | 0.16 |
| | | High performing peers | 0.32 | 0.33 | 0.00 | 1.00 | 0.15 |

**Table 3 Features** Overview over investigated features including descriptive statistics.
